# Supplementary material for: Possible quantum paramagnetism in compressed Sr$_2$IrO$_4$
Source: arXiv:1911.09786 ancillary file (2020-02-13)
Supplement: Supplementary file 1 [file supplemental.pdf]

# Supplemental material for: Possible quantum paramagnetism in compressed $\text{Sr}_2\text{IrO}_4$

D. Haskel,<sup>1,\*</sup> G. Fabbri,<sup>1,†</sup> J. H. Kim,<sup>1</sup> L. S. I. Veiga,<sup>1,2,3</sup> J. R. L. Mardegan,<sup>1,3</sup> C. A. Escanhoela Jr.,<sup>1,2</sup> S. Chikara,<sup>1</sup> V. Struzhkin,<sup>4</sup> T. Senthil,<sup>5</sup> B. J. Kim,<sup>6,7</sup> G. Cao,<sup>8</sup> and J. W. Kim<sup>1</sup>

<sup>1</sup>Advanced Photon Source, Argonne National Laboratory, Argonne, Illinois 60439, USA

<sup>2</sup>Brazilian Synchrotron Light Laboratory (LNLS), Campinas, SP 13083-970, Brazil

<sup>3</sup>Instituto de Física “Gleb Wataghin”, Universidade Estadual de Campinas, Campinas, SP 13083-859, Brazil

<sup>4</sup>Geophysical Laboratory, Carnegie Institution of Washington, Washington, DC 20015, USA

<sup>5</sup>Department of Physics, Massachusetts Institute of Technology, Cambridge, Massachusetts 02139, USA

<sup>6</sup>Max-Planck-Institut für Festkörperforschung, Heisenbergstr. 1, Stuttgart D-70569, Germany

<sup>7</sup>Department of Physics, Pohang University of Science and Technology, Pohang 790-784, Republic of Korea

<sup>8</sup>Department of Physics, University of Colorado, Boulder, Colorado 80309, USA

(Dated: November 15, 2019)

## EXPERIMENTAL METHODS

X-ray resonant magnetic scattering (XRMS) measurements in the diamond anvil cell (DAC) were carried out at beamlines 4-ID-D and 6-ID-B of the Advanced Photon Source at Argonne National Laboratory. Both reflection (Bragg) and transmission (Laue) scattering geometries were used with panoramic [1] and Merrill-Basset [2] type DACs (Fig. S1), using regular and Bohler-Almax anvils, respectively ( $T = 5\text{--}10\text{ K}$ ). Single crystals grown at both the University of Kentucky and Argonne National Laboratory with platelet shape dimensions  $\approx 50 \times 50 \times 20\text{ }\mu\text{m}^3$  were used in the measurements. Crystals with  $c$ -axis oriented out (in) plane of the platelet were used for Bragg reflection (Laue) scattering geometries. Diamond culet diameter was either 300 or 500  $\mu\text{m}$ , Neon used as pressure transmitting medium, and Rhenium metal as gasket material. Pressure was calibrated *in-situ* using the P-V equation of state of a Au or Ag metal foil loaded in the sample chamber [3]. Results from experiments using different scattering geometries and different crystals were consistent.

X-ray magnetic circular dichroism (XMCD) measure-

ments were carried out at beamline 4-ID-D using a helicity-modulation technique in transmission geometry [4]. A superconducting magnet (6.5 T) with a bore large enough to accept a membrane-driven CuBe DAC was used ( $T = 1.5\text{--}300\text{ K}$ ). Powder samples obtained from single crystals were primarily used for these measurements. A partially perforated anvil, opposite a mini-anvil mounted on a fully perforated anvil, was used to minimize x-ray attenuation [5, 6]. Diamond culet diameter was 450  $\mu\text{m}$ , Neon used as pressure medium and Rhenium metal used as gasket material. Pressure was calibrated *in-situ* using an online Ruby fluorescence system that inserts into the (reentrant) radial bore of the split-coil superconducting magnet [7].

## OCTAHEDRAL ROTATIONS AND CRYSTAL STRAIN UNDER PRESSURE

The staggered rotations of  $\text{IrO}_6$  octahedra around the  $c$ -axis present in the  $I4_1/acd$  tetragonal space group of  $\text{Sr}_2\text{IrO}_4$  (Sr-214) [8–10], and related periodic pattern of displacements of oxygen ions, give rise to superlattice reflections that can be probed with single crystal

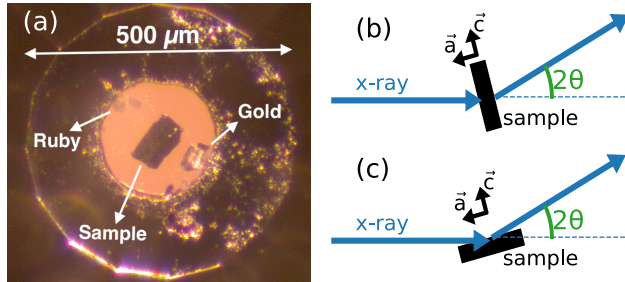

FIG. S1. (a) Optical image of typical DAC sample chamber used in the XRMS experiments. Ruby fluorescence is used to calibrate pressure during gas loading while the lattice constant of gold is used as manometer during the XRMS measurements. (b,c) Schematics of the transmission (Laue) and reflection scattering geometries used in the XRMS experiments.

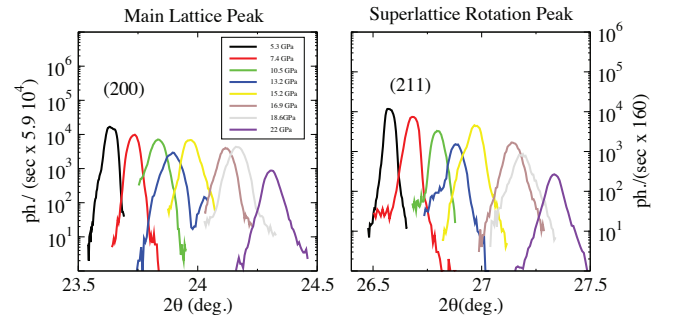

FIG. S2. Single crystal x-ray diffraction measurements of superlattice Bragg peak (211) arising from octahedral rotations together with measurements of nearby main lattice peak (200) ( $T = 5\text{ K}$ ).

diffraction. A single crystal with approximate dimensions  $97 \times 86 \times 20 \mu\text{m}^3$  ( $c$ -axis out of plane) was loaded into a  $210 \mu\text{m}$  diameter sample chamber drilled in a stainless steel gasket pre-indented to  $80 \mu\text{m}$  thickness with  $450 \mu\text{m}$  culet diameter diamond anvils. XRD measurements were carried out at  $T = 5 \text{ K}$  using  $11.190 \text{ keV}$  x-rays. A  $12.5 \mu\text{m}$ -thick silver foil was loaded into the sample chamber for in-situ pressure calibration using the known response of silver's lattice parameter to pressure at low temperature [3]. Pressure medium was 4:1 methanol-ethanol mixture.

Figure S2 shows the evolution with pressure of  $\theta - 2\theta$  scans for (211) superlattice peak and the nearby (200) main lattice peak. The (211) reflection is  $\sim 400$  times weaker than the (200) main lattice peak as a result of the low scattering power of (low- $Z$ ) oxygen ions. The integrated intensities of superlattice and main Bragg peaks roughly follow each other and their ratio does not change by more than a factor of two over the entire pressure range. The data clearly shows that the pattern of octahedral rotations does not change, and that the rotation angle remains sizable. A quantitative measurement of the rotation angle from the measured intensity is not possible since small distortions in oxygen positions can preferentially reduce the intensity of the superlattice peak relative to the main lattice peak. However we can put a lower bound on the size of the distortion by noting that the intensity of the rotation peak scales with  $\theta^2$ , where  $\theta$  is the rotation angle ( $11.5^\circ$  at ambient pressure). Since the ratio of intensities between (211) and (200) peaks does not decrease beyond a factor of 2, we can place a lower limit of  $11.5/\sqrt{2} = 8^\circ$  for the rotation angle at the highest pressure. We note that the data cannot rule out a small increase in rotation angle under pressure due to intensity reduction of superlattice peak as a result of small local distortions away from a coherent rotation pattern, as discussed above. That the  $a$ -axis lattice parameter has a slightly larger compressibility than the  $c$ -axis [11, 12] suggests that the rotation angle may actually increase with pressure, as suggested by recent density functional theory calculations [12].

An independent set of measurements was carried out on a second crystal with in-plane  $c$ -axis orientation using Neon as pressure-transmitting medium. For this test Bohler-Almax diamond anvils with  $500 \mu\text{m}$  culet diameter were used and a crystal with dimensions  $50 \times 100 \times 20 \mu\text{m}^3$  was loaded into a  $300 \mu\text{m}$  hole in a stainless steel gasket pre-indented to  $80 \mu\text{m}$ . The final sample chamber diameter after gas loading was  $220 \mu\text{m}$ . In this experiment the (1,2,11) superlattice peak and the nearby (1,1,10) main lattice peak were measured up to  $23 \text{ GPa}$  at  $T = 10 \text{ K}$ . The superlattice peak is  $\sim 440$  times weaker than the main lattice peak but remains strong to the highest pressure confirming that the pattern of rotations remains unchanged. At  $23 \text{ GPa}$  the ratio of integrated intensities between superlattice and main lattice Bragg peaks is only

$1.6$  smaller than its value at low pressures placing a lower limit for the rotation angle at  $11.5/\sqrt{1.6} = 9.1^\circ$ . We conclude that, at least to  $23 \text{ GPa}$ , the pattern of octahedral rotations is preserved and that the octahedral rotation angle is at least  $8$ - $9^\circ$  if not larger. A precise determination of the evolution of the rotation angle with pressure requires structural refinements of comprehensive single crystal diffraction data. Due to the weak x-ray scattering power of light O atoms in the presence of strong scattering from heavy Ir/Sr atoms, neutron powder diffraction measurements to  $25 \text{ GPa}$  may be required to quantify oxygen displacement.

Rocking curves show that the crystal mosaic width does not increase by more than a factor of two over the entire pressure range and remains in the  $0.1$ - $0.2^\circ$  range at all pressures. Crystal strain induced by pressure gradients can be estimated from Bragg peak broadening in  $\theta - 2\theta$  scans. For the  $a$ -axis the incremental broadening is  $\Delta(2\theta) \leq 0.02^\circ$  or a strain value of  $(a_H - a_L)/a_L = a_L^2 \sin(2\theta) \Delta\theta / (2\lambda^2) \sim 0.1\%$  ( $a_H$  and  $a_L$  are lattice parameters at highest and lowest pressure values, respectively). Based on the pressure dependence of the (200) Bragg angle ( $0.019^\circ/\text{GPa}$ ) this corresponds to a pressure gradient of  $\sim 0.5 \text{ GPa}$  at the highest pressure of  $23 \text{ GPa}$ .

## EXTRACTING $T_N$ FROM THE PRESSURE- AND TEMPERATURE-DEPENDENT XMCD DATA

As seen in Fig. 2(b) of the main manuscript, the collapse of magnetic order as a function of pressure (at  $11 \text{ K}$ ) and temperature (at  $1 \text{ bar}$ ) have identical behavior when plotted as a function of reduced pressure/temperature. Therefore, in order to extract the pressure dependence of  $T_N$ , we used the functional form of the  $T$ -dependent XMCD collected at  $0.8 \text{ T}$  and  $1 \text{ bar}$  as a reference [Fig. S3(a)] [11]. This reference was fitted to the pressure dependence at low temperatures [Fig. S3(b-d)], and to the temperature dependence at selected pressures [Fig. S3(e-h)]. For the latter, the experimental points correspond to the averaged XMCD within a pressure window of  $\pm 1 \text{ GPa}$ .

## CONVERSION OF XMCD DATA TO MAGNETIC SUCCEPTIBILITY

The susceptibility of a magnetic material with local exchange interactions but lacking spontaneous order due to fluctuations is given by the Curie-Weiss law  $\chi = C/(T - \theta_{CW})$  with  $\chi = M/H$ ,  $C$  the Curie constant, and  $\theta_{CW}$  the Curie-Weiss temperature, the latter a measure of the strength and sign of local exchange interactions. The element specific XMCD technique is one of the only ways to probe the small net magnetization of

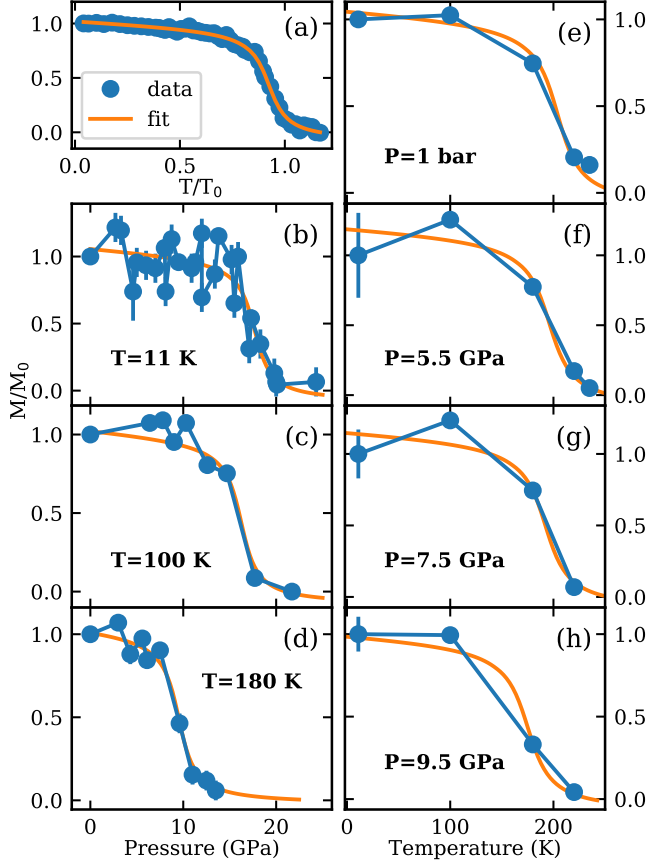

FIG. S3. (a) Temperature dependence of the Ir  $L_3$  XMCD at 1 bar and 0.8 T from Ref. 11. The data was modeled using an arctangent step function, which was then used as a reference to retrieve  $T_N$  as a function of pressure. (b-d) Isothermal Ir  $L_3$  XMCD data as a function of pressure. (e-h) Isobaric Ir  $L_3$  XMCD as a function of temperature.

Sr-214 at high pressures and low temperature. In order to compute susceptibility from XMCD data, the sample magnetization is obtained with the use of sum rules [13, 14]. As reported previously the XMCD signals at the Ir  $L$ -edges of  $\text{Ir}^{4+}$  ions in  $J_{\text{eff}} = 1/2$ -like electronic configuration display a large asymmetry between  $L_3$  and  $L_2$  edges due to a sizable orbital moment contribution to the total magnetic moment ( $L_3$ -edge XMCD signal 9-20 times larger than the  $L_2$ -edge XMCD [11, 15, 16]). The derivation of total magnetic moment from XMCD sum rules is therefore dominated by the XMCD signal at the  $L_3$  edge.

At ambient pressure and low temperature sum rules yield a net magnetic moment of  $0.045(4)\mu_B/\text{Ir}$  in the ordered state of Sr-214 in good agreement with results from magnetometry for which a powder average of single crystal data yields  $0.05\mu_B/\text{Ir}$  [11, 17, 18]. The corresponding  $L_3$  XMCD signal, properly normalized to the

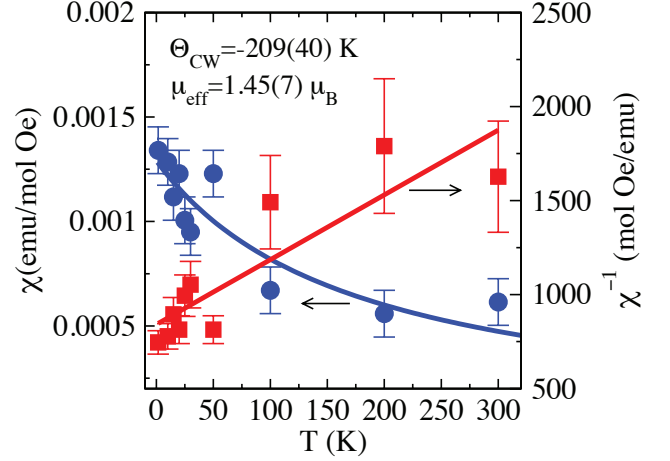

FIG. S4. Temperature dependence of DC magnetic susceptibility at  $P=35$  GPa and  $H= 6$  T, together with fits to a Curie-Weiss law used to determine values of  $\theta_{CW}$  and  $\mu_{\text{eff}}$ .

absorption edge jump, is 3%. It has been shown, based on measurements of the isotropic branching ratio[11], that Sr-214 retains the ambient pressure  $J_{\text{eff}} = 1/2$ -like configuration up to about 40 GPa where a structural transition takes place[12]. Therefore we can assume that the ratio of  $L_3$  to  $L_2$  XMCD intensities remains unchanged to 35 GPa. The temperature-dependence of the  $L_3$  edge XMCD signal at  $P=35$  GPa can therefore be converted to sample magnetization using the scaling derived above. For example at  $T=1.5$  K,  $H=6$  T, and  $P=35$  GPa the 1% XMCD signal corresponds to  $0.015\mu_B/\text{Ir}$  or a susceptibility  $\chi = M/H = 1.4 \times 10^{-3}$  emu/(mol Oe). Figure S4 shows fits to the temperature dependence of the direct and inverse susceptibility from which values of  $\theta_{CW} = -209(40)$  K and effective moment  $\mu_{\text{eff}} = \sqrt{8C} = 1.45(7)\mu_B$  are obtained.

\* haskel@anl.gov

† gfabbris@anl.gov

- [1] A. G. Gavriluk, A. A. Mironovich, and V. V. Struzhkin, "Miniature diamond anvil cell for broad range of high pressure measurements," *Review of Scientific Instruments* **80**, 043906 (2009).
- [2] Yejun Feng, R. Jaramillo, Jiyang Wang, Yang Ren, and T. F. Rosenbaum, "Invited Article: High-pressure techniques for condensed matter physics at low temperature," *Review of Scientific Instruments* **81**, 041301 (2010).
- [3] W. B. Holzapfel, M. Harwig, and W. Sievers, "Equations of State for Cu, Ag, and Au for Wide Ranges in Temperature and Pressure up to 500 GPa and Above," *Journal of Physical and Chemical Reference Data* **30**, 515 (2001).
- [4] Motohiro Suzuki, Naomi Kawamura, Masaichiro Mizumaki, Akiri Urata, Hiroshi Maruyama, Shunji Goto, and Tetsuya Ishikawa, "Helicity-Modulation Technique Using

- Diffraction Phase Retarder for Measurements of X-ray Magnetic Circular Dichroism,” *Japanese Journal of Applied Physics* **37**, L1488–L1490 (1998).
- [5] D. Haskel, Y. C. Tseng, J. C. Lang, and S. Sinogeikin, “Instrument for x-ray magnetic circular dichroism measurements at high pressures,” *Review of Scientific Instruments* **78**, 083904 (2007).
- [6] Daniel Haskel, Y. C. Tseng, N. M. Souza-Neto, J. C. Lang, S. Sinogeikin, Ya Mudryk, K. A. Gschneidner, and V. K. Pecharsky, “Magnetic spectroscopy at high pressures using X-ray magnetic circular dichroism,” *High Pressure Research* **28**, 185–192 (2008).
- [7] K. Syassen, “Ruby under pressure,” *High Pressure Research* **28**, 75–126 (2008).
- [8] Feng Ye, Songxue Chi, Bryan C. Chakoumakos, Jaime A. Fernandez-Baca, Tongfei Qi, and G. Cao, “Magnetic and crystal structures of  $\text{Sr}_2\text{IrO}_4$ : A neutron diffraction study,” *Physical Review B* **87**, 140406 (2013).
- [9] M K Crawford, M A Subramanian, R. L. Harlow, J. A. Fernandez-Baca, Z R Wang, and D C Johnston, “Structural and magnetic studies of  $\text{Sr}_2\text{IrO}_4$ ,” *Physical Review B* **49**, 9198–9201 (1994).
- [10] Q. Huang, J.L. Soubeyroux, O. Chmaissem, I. Natali Sora, A. Santoro, R.J. Cava, J.J. Krajewski, and W.F. Peck, “Neutron Powder Diffraction Study of the Crystal Structures of  $\text{Sr}_2\text{RuO}_4$  and  $\text{Sr}_2\text{IrO}_4$  at Room Temperature and at 10 K,” *Journal of Solid State Chemistry* **112**, 355–361 (1994).
- [11] D. Haskel, G. Fabbri, Mikhail Zhernenkov, P. P. Kong, C. Q. Jin, G. Cao, and M. van Veenendaal, “Pressure Tuning of the Spin-Orbit Coupled Ground State in  $\text{Sr}_2\text{IrO}_4$ ,” *Physical Review Letters* **109**, 027204 (2012).
- [12] K. Samanta, F. M. Ardito, N. M. Souza-Neto, and E. Granado, “First-order structural transition and pressure-induced lattice/phonon anomalies in  $\text{Sr}_2\text{IrO}_4$ ,” *Physical Review B* **98**, 094101 (2018).
- [13] B. T. Thole, P. Carra, F. Sette, and G. van der Laan, “X-ray circular dichroism as a probe of orbital magnetization,” *Physical Review Letters* **68**, 1943–1946 (1992).
- [14] Paolo Carra, B. T. Thole, Massimo Altarelli, and Xindong Wang, “X-ray circular dichroism and local magnetic fields,” *Physical Review Letters* **70**, 694–697 (1993).
- [15] M. A. Laguna-Marco, D. Haskel, N. Souza-Neto, J. C. Lang, V. V. Krishnamurthy, S. Chikara, G. Cao, and M. van Veenendaal, “Orbital Magnetism and Spin-Orbit Effects in the Electronic Structure of  $\text{BaIrO}_3$ ,” *Physical Review Letters* **105**, 216407 (2010).
- [16] T. Takayama, A. Kato, R. Dinnebier, J. Nuss, H. Kono, L. S. I. Veiga, G. Fabbri, D. Haskel, and H. Takagi, “Hyperhoneycomb Iridate  $\beta$  –  $\text{Li}_2\text{IrO}_3$  as a Platform for Kitaev Magnetism,” *Physical Review Letters* **114**, 077202 (2015).
- [17] M. Ge, T. F. Qi, O. B. Korneta, D. E. De Long, P. Schlottmann, W. P. Crummett, and G. Cao, “Lattice-driven magnetoresistivity and metal-insulator transition in single-layered iridates,” *Physical Review B* **84**, 100402 (2011).
- [18] S. Chikara, O. Korneta, W. P. Crummett, L. E. DeLong, P. Schlottmann, and G. Cao, “Giant magnetoelectric effect in the  $J_{eff} = \frac{1}{2}$  Mott insulator  $\text{Sr}_2\text{IrO}_4$ ,” *Physical Review B* **80**, 140407 (2009).
